# Supplementary material for: Nonequilibrium phonon backaction on the current noise in atomic-sized junctions
Source: arXiv:1105.3912 source file (2011-09-16)
Supplement: Supplementary file 1 [file Supplementary_note.pdf]

# Supplementary Material for "Non-equilibrium phonon back-action on the current noise in atomic-sized junctions"


Tomáš Novotný,[1,2] Federica Haupt,[3,4] and Wolfgang Belzig[4]

[1]*Department of Condensed Matter Physics, Faculty of Mathematics and Physics, Charles University in Prague, Ke Karlovu 5, CZ-121 16 Praha 2, Czech Republic*
[2]*Institut NÉEL, CNRS and Université Joseph Fourier, BP 166, F-38042 Grenoble Cedex 9, France*
[3]*Institut für Theorie der statistischen Physik, RWTH Aachen University, D-52056 Aachen, Germany*
[4]*Fachbereich Physik, Universität Konstanz, D-78457 Konstanz, Germany*



(Dated: July 19, 2011)



In this supplementary material we consider explicitly the effects of finite phonon-damping due to coupling to an external heat bath. In addition, we give details of the simple tight binding model used to study the noise in atomic gold wires with unit transmission (see Fig. 1 in the main text), and use the same model to exemplify the effects of external phonon damping.



PACS numbers: 72.70.+m, 72.10.Di, 85.65.+h, 73.63.-b


### External phonon damping

In the spirit of the Caldeira-Legget model [1], dissipative effects due to an external heat bath can be addressed at the Hamiltonian level in terms of a linear coupling between the molecular phonon and a bath of harmonic oscillators. In other words, in the presence of an external bath the total Hamiltonian of the system becomes $\hat{H} = \hat{H}_C + \hat{H}_{L,R} + \hat{H}_T + \hat{H}_B + \hat{H}_{\rm phB}$, where $\hat{H}_C$, $\hat{H}_{L,R}$, and $\hat{H}_T$ are defined as in the main text, and

$$\hat{H}_B = \sum_j \Omega_j \hat{a}_j^\dagger \hat{a}_j,$$
$$\hat{H}_{\rm phB} = \sum_j \chi_j (\hat{a}_j^\dagger + \hat{a}_j)(\hat{b}^\dagger + \hat{b}),$$

where $\hat{a}_j^\dagger(\hat{a}_j)$ are the creation (annihilation) operators of the bosonic bath modes, and $\chi_j$ defines the phonon-bath interaction.

In the presence of both e-ph coupling *and* of the external bath, the dressed phonon Green's function $\check{D}_\lambda$ is given by the Dyson equation

$$\check{D}_\lambda(\varepsilon) = \frac{2\Omega}{\mathcal{D}_\lambda(\varepsilon)} \begin{pmatrix} \varepsilon^2 - \Omega^2 + 2\Omega\Pi^{++}_{\rm tot} & 2\Omega\Pi^{-+}_{\rm tot} \\ 2\Omega\Pi^{+-}_{\rm tot} & -\varepsilon^2 + \Omega^2 + 2\Omega\Pi^{--}_{\rm tot} \end{pmatrix},$$

where $\mathcal{D}_\lambda(\varepsilon) = \left(\varepsilon^2 - \Omega^2 + 2\Omega\Pi^{++}_{\rm tot}\right)\left(\varepsilon^2 - \Omega^2 - 2\Omega\Pi^{--}_{\rm tot}\right) + 4\Omega^2\Pi^{-+}_{\rm tot}\Pi^{+-}_{\rm tot}$ and $\check{\Pi}_{\rm tot} = \check{\Pi}_\lambda + \check{\Pi}_B$ is the total self-energy of the phonon, with $\check{\Pi}_\lambda$ the self-energy due to the electron-phonon interaction (as given by Eq. (1) in the main text), and $\check{\Pi}_B$ the one due to coupling to the external bath

$$\Pi_B^{-+}(\varepsilon) = -2in_B(\varepsilon)\mathrm{sign}(\varepsilon)J(|\varepsilon|),$$
$$\Pi_B^{+-}(\varepsilon) = -2i[1 + n_B(\varepsilon)]\mathrm{sign}(\varepsilon)J(|\varepsilon|),$$
$$\Pi_B^{\pm\pm}(\varepsilon) = -i[1 + 2n_B(\varepsilon)]\mathrm{sign}(\varepsilon)J(|\varepsilon|) \mp \mathcal{P}\sum_j \frac{2\chi_j^2\Omega_j}{\varepsilon^2 - \Omega_j^2},$$

where $J(\varepsilon) = \pi\sum_j \chi_j^2 \delta(\varepsilon - \Omega_j)$ is the bath spectral density and $n_B(\varepsilon) = (e^{\beta\varepsilon} - 1)^{-1}$ the Bose distribution.

In the limit of *weak coupling* to both the tunneling electrons and to the external bath, the dressed phonon Green's function can be approximated by the kinetic-limit expression (see discussion below Eq. (3) in the main text)

$$\check{D}_\lambda(\varepsilon) = \begin{pmatrix} \mathcal{P}\frac{2\Omega}{\varepsilon^2 - \Omega^2} & 0 \\ 0 & -\mathcal{P}\frac{2\Omega}{\varepsilon^2 - \Omega^2} \end{pmatrix} - 2\pi i \sum_{s=\pm} \delta(\varepsilon + s\Omega)\check{\mathcal{N}}_\lambda(\varepsilon), \tag{1}$$

where

$$\check{\mathcal{N}}_\lambda(\varepsilon) = \frac{i}{\sqrt{\xi_{\rm tot}(\varepsilon)}} \begin{pmatrix} \frac{\Pi^{--}_{\rm tot}(\varepsilon) + \Pi^{++}_{\rm tot}(\varepsilon)}{2} & \Pi^{-+}_{\rm tot}(\varepsilon) \\ \Pi^{+-}_{\rm tot}(\varepsilon) & \frac{\Pi^{--}_{\rm tot}(\varepsilon) + \Pi^{++}_{\rm tot}{\rm tot}(\varepsilon)}{2} \end{pmatrix},$$

with $\xi_{\rm tot}(\varepsilon) = 4\Pi^{-+}_{\rm tot}(\varepsilon)\Pi^{+-}_{\rm tot}(\varepsilon) - (\Pi^{++}_{\rm tot}(\varepsilon) + \Pi^{--}_{\rm tot}(\varepsilon))^2$.

At $\lambda = 0$, the generalized occupation $\check{\mathcal{N}}_\lambda$ reduces to

$$\check{\mathcal{N}}_{\lambda=0}(\varepsilon) = \begin{pmatrix} \bar{N}(\varepsilon) + 1/2 & \bar{N}(\varepsilon) \\ \bar{N}(\varepsilon) + 1 & \bar{N}(\varepsilon) + 1/2 \end{pmatrix},$$

where

$$\bar{N}(\varepsilon) \equiv \frac{i\Pi^{-+}_{\lambda=0}(\varepsilon) + 2n_B(\varepsilon)\mathrm{sign}(\varepsilon)J(|\varepsilon|)}{2|\mathrm{Im}\Pi^R(\varepsilon) - \mathrm{sign}(\varepsilon)J(|\varepsilon|)|}, \tag{2}$$

is the *non-equilibrium* phonon occupation number ($\Pi^R(\varepsilon) \equiv \Pi^{--}_{\lambda=0}(\varepsilon) - \Pi^{-+}_{\lambda=0}(\varepsilon)$ as in the main text).

A few observations are now in order: if the coupling to the external bath is much stronger than the e-ph interaction ($J(\Omega) \gg \gamma_{\rm eph}\Omega$), the generalized phonon-occupation becomes independent of the counting field $\lambda$, and $\check{D}_\lambda(\varepsilon)$ reduces to the standard expression for the Green's functions of a free thermal phonon. Following Ref. [2], we call this the *externally damped limit.* In the opposite case ($J(\Omega) \to 0$), which we then call *externally undamped limit*, $\check{\mathcal{N}}_\lambda$ becomes independent of the strength of the e-ph coupling. Physically this means that if the phonon is not coupled to any external bath, then even an infinitesimally weak e-ph interaction eventually gives rise to a

stationary state with a strongly non equilibrium phonon occupation [3].

Concerning the effects of phonon heating on the current noise $S$, it is important to notice that the phonon self-energy due the external heath bath is independent of the counting field $\lambda$. It is easy to show that also in the presence of external phonon damping, the lowest order correction to the current noise due to e-ph coupling can be split into two parts $S_{\rm eph} = S_{\rm av} + S_{\rm ba}$, where $S_{\rm av}$ is simply given by the result of Ref. [4] with the thermal phonon occupation replaced by the non-equilibrium one, $n_B(\Omega) \to \bar{N} \equiv \bar{N}(\Omega)$, with $\bar{N}(\varepsilon)$ as given in Eq. (2), and

$$\begin{aligned}\frac{S_{\rm ba}}{e^2/\hbar} = &-\frac{\Pi'_{++}+\Pi'_{--}-\Pi'_{+-}-\Pi'_{-+}}{|{\rm Im}\Pi^R(\Omega)|+J(\Omega)} \\ &\times\Big\{\bar{N}(\bar{N}+1)(\Pi'_{++}+\Pi'_{--}-\Pi'_{+-}-\Pi'_{-+}) \\ &+\big(\bar{N}+\tfrac{1}{2}\big)(\Pi'_{+-}-\Pi'_{-+})-\tfrac{1}{2}(\Pi'_{+-}+\Pi'_{-+})\Big\},\end{aligned} \tag{3}$$

with $\Pi'_{\alpha\beta} \equiv \frac{\partial}{\partial\lambda}\Pi^{\alpha\beta}_{\lambda}(\Omega)\big|_{\lambda=0}$. This expression is valid for an *arbitrary* junction with weak e-ph coupling and weak coupling to the external bath (kinetic limit).

While Eq. (3) can in general be evaluated only numerically, analytic progress can be made in the extended wide band approximation (eWBA) [4, 5], which is applicable if the electronic structure is slowly varying over the relevant energy range around the Fermi level (typically several multiples of the phonon energy). In this case, all the terms appearing in Eq. (3) can be calculated analytically. At zero temperature, the resulting expressions are:

$$\Pi'_{+-}+\Pi'_{-+} = \alpha_1 eV + \alpha_2\,{\rm sign}(eV){\rm min}(|eV|,\Omega), \tag{4a}$$
$$\Pi'_{+-}-\Pi'_{-+} = (\alpha_1+\alpha_2){\rm sign}(eV){\rm min}(|eV|,\Omega), \tag{4b}$$
$$\Pi'_{++}+\Pi'_{--}-\Pi'_{+-}-\Pi'_{-+} = \alpha_3 eV, \tag{4c}$$
$$\Pi^{-+}_{\lambda=0}(\Omega) = \alpha_4(|eV|-\Omega)\theta(|eV|-\Omega), \tag{4d}$$
$${\rm Im}\Pi^R(\Omega) = \alpha_5\Omega, \tag{4e}$$
$$\bar{N} = \frac{i\alpha_4(|eV|-\Omega)\theta(|eV|-\Omega)}{2|\alpha_5|\Omega+J(\Omega)}, \tag{4f}$$

with

$$\begin{aligned}\alpha_1 =& \frac{i}{2\pi}{\rm Tr}\big\{\mathbf{M}\mathbf{A}_L\mathbf{M}\mathbf{A}_R\mathbf{\Gamma}_L\mathbf{A}_R - \mathbf{M}\mathbf{A}_R\mathbf{M}\mathbf{A}_L\mathbf{\Gamma}_L\mathbf{A}_L \\ &- \mathbf{M}\mathbf{A}_R\mathbf{M}\mathbf{g}^r\mathbf{\Gamma}_L\mathbf{g}^a - 2i\mathbf{M}\mathbf{A}_R\mathbf{M}\mathbf{A}_L\mathbf{\Gamma}_L\mathbf{g}^a + H.c\big\}, \\ \alpha_2 =& \frac{i}{2\pi}{\rm Tr}\big\{\mathbf{M}(\mathbf{A}_L-\mathbf{A}_R)\mathbf{M}\big[\mathbf{A}_R\mathbf{\Gamma}_L(\mathbf{A}_L+i\mathbf{g}^a)+H.c\big]\big\}, \\ \alpha_3 =& \frac{i}{2\pi}{\rm Tr}\big\{2\mathbf{M}\mathbf{g}^r\mathbf{M}\mathbf{A}_R\mathbf{\Gamma}_L\mathbf{g}^r + \mathbf{M}\mathbf{A}_R\mathbf{M}\mathbf{g}^a\mathbf{\Gamma}_L\mathbf{g}^r + H.c\big\}, \\ \alpha_4 =& -\frac{i}{2\pi}{\rm Tr}\big\{\mathbf{M}\mathbf{A}_L\mathbf{M}\mathbf{A}_R\big\}, \\ \alpha_5 =& -\frac{1}{4\pi}{\rm Tr}\big\{\mathbf{M}(\mathbf{A}_L+\mathbf{A}_R)\mathbf{M}(\mathbf{A}_L+\mathbf{A}_R)\big\}.\end{aligned}$$

These quantities depend only on the properties of the system at the Fermi level and can in principle be evaluated by *ab-initio* calculations. The general eWBA expressions at finite temperature can be found in the associated `Mathematica` notebook.

### Simple model for an atomic gold chain

As a simple illustration of our method, we study the noise in an atomic gold chain described in terms of a simple tight-binding model [2, 3, 5–7]. We consider a N-atoms wire, coupled to two fixed electrodes. Each electrode is represented by a single electronic orbital, which we think of as being connected to the next layer of the electrode. In total, the chain is then formed by N+2 sites, with onsite energy $\varepsilon_0$, and inter-site hopping $t$. As an example, taking for definiteness $N = 2$, the Hamiltonian of the wire reads

$$\mathbf{H}_c = \begin{pmatrix}\varepsilon_0 & t & 0 & 0\\ t & \varepsilon_0 & t & 0\\ 0 & t & \varepsilon_0 & t\\ 0 & 0 & t & \varepsilon_0\end{pmatrix}. \tag{5}$$

The coupling to the "bulk" electrode, introduce a finite line-width in the outermost sites of the chain

$$\mathbf{\Gamma}_L = \begin{pmatrix}\gamma_L & 0 & 0 & 0\\ 0 & 0 & 0 & 0\\ 0 & 0 & 0 & 0\\ 0 & 0 & 0 & 0\end{pmatrix}, \quad \mathbf{\Gamma}_R = \begin{pmatrix}0 & 0 & 0 & 0\\ 0 & 0 & 0 & 0\\ 0 & 0 & 0 & 0\\ 0 & 0 & 0 & \gamma_R\end{pmatrix}, \tag{6}$$

which in the eWBA we take to be energy independent. The retarded Green's function of the chain is readily given by $\mathbf{g}^r(\varepsilon) = [\varepsilon\mathbf{1} - \mathbf{H}_c - \mathbf{\Sigma}^r_T]^{-1}$, with $\mathbf{\Sigma}^r_T = -i(\mathbf{\Gamma}_L + \mathbf{\Gamma}_R)/2$ the self energy due to coupling to leads. It is well established that atomic gold wires have one almost perfectly transmitting channel at the Fermi energy [8]. To achieve unit transmission in our model, we set $\varepsilon_0 = E_F = 0$ and $\gamma_L = \gamma_R = 2t$.

We consider here coupling to a phonon mode with alternating bond-length (ABL) character, which is known to be the dominant inelastic scattering mechanism in Au wires [2]. For simplicity, we assume the e-ph coupling matrix to be of the form

$$\mathbf{M} = \begin{pmatrix}0 & m & 0 & 0\\ m & 0 & -m & 0\\ 0 & -m & 0 & m\\ 0 & 0 & m & 0\end{pmatrix}. \tag{7}$$

With these definitions, the coefficients $\alpha_1, \ldots, \alpha_5$ introduced in Eq. (4) take on the explicit form $\alpha_1 = i\gamma_{\rm eph}/\pi, \alpha_2 = 0, \alpha_3 = -i\gamma_{\rm eph}/\pi, \alpha_4 = -i\gamma_{\rm eph}/2\pi, \alpha_5 = -\gamma_{\rm eph}/2\pi$, with $\gamma_{\rm eph} = (N-1)^2m^2/t^2$ the dimensionless e-ph coupling in the chain.

With this concrete model in mind, we study the effects of dissipation due to an external bath on the current noise in an atomic wire. The results are summarized in Fig. 1,

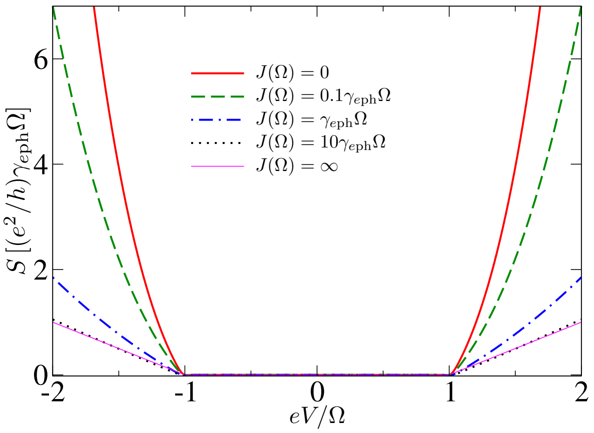


FIG. 1. Effects of external phonon damping on the current noise in an atomic gold wire. We consider here a perfectly transmitting gold wire in the presence of an alternating-bond-length phonon mode at zero temperature [2, 5]. In this case $S_{\mathrm{elastic}} = 0$. Different curves correspond to different strengths of the coupling to the external phonon bath. The cases $J(\Omega) = 0$ and $J(\Omega) = \infty$ corresponds to the externally undamped and externally damped limits, respectively.

where we plot the total noise $S = S_{\mathrm{av}} + S_{\mathrm{ba}}$ through the chain for different values of phonon-bath coupling, which is parametrized by the bath spectral density at the phonon frequency $J(\Omega)$. Not surprisingly, a finite degree of equilibration simply interpolates between the two limiting cases of externally undamped ($J(\Omega) = 0$) and externally damped phonon ($J(\Omega) = \infty$).

[1] A. O. Caldeira and A. J. Leggett, Annals of Physics, **149**, 374 (1983).

[2] T. Frederiksen, M. Brandbyge, N. Lorente, and A.-P. Jauho, Phys. Rev. Lett., **93**, 256601 (2004).

[3] J. K. Viljas, J. C. Cuevas, F. Pauly, and M. Häfner, Phys. Rev. B, **72**, 245415 (2005).

[4] F. Haupt, T. Novotný, and W. Belzig, Phys. Rev. B, **82**, 165441 (2010).

[5] M. Paulsson, T. Frederiksen, and M. Brandbyge, Phys. Rev. B, **72**, 201101 (2005).

[6] L. de la Vega, A. Martín-Rodero, N. Agraït, and A. L. Yeyati, Phys. Rev. B, **73**, 075428 (2006).

[7] T. Frederiksen, M. Brandbyge, A.-P. Jauho, and N. Lorente, J. Comput. Electron., **3**, 423 (2004).

[8] N. Agraït, A. L. Yeyati, and J. M. van Ruitenbeek, Phys. Rep., **377**, 81 (2003).
